# Supplementary material for: Electrical percolation in metal wire network based strain sensors
Source: arXiv:1902.03746 source file (2019-02-11)
Supplement: Supplementary file 1 [file Supplementary_Material.pdf]

Supplementary Material

# Electrical percolation in metal wire network based strain sensors

Ankush Kumar[1]

*Chemistry and Physics of Materials Unit, Jawaharlal Nehru Centre for Advanced Scientific Research,560064, Bangalore, India*[a)]

Keywords: Strain sensors, Metal wire network, Electrical percolation, Stretchable Electronics, Transparent conductors.

[a)]Electronic mail: ankush.science@gmail.com; Present Adress: Department of Mathematics, University of Pittsburgh.

## I. RESISTANCE VARIATION FOR AN ARBITRORY DIRECTION OF STRAIN

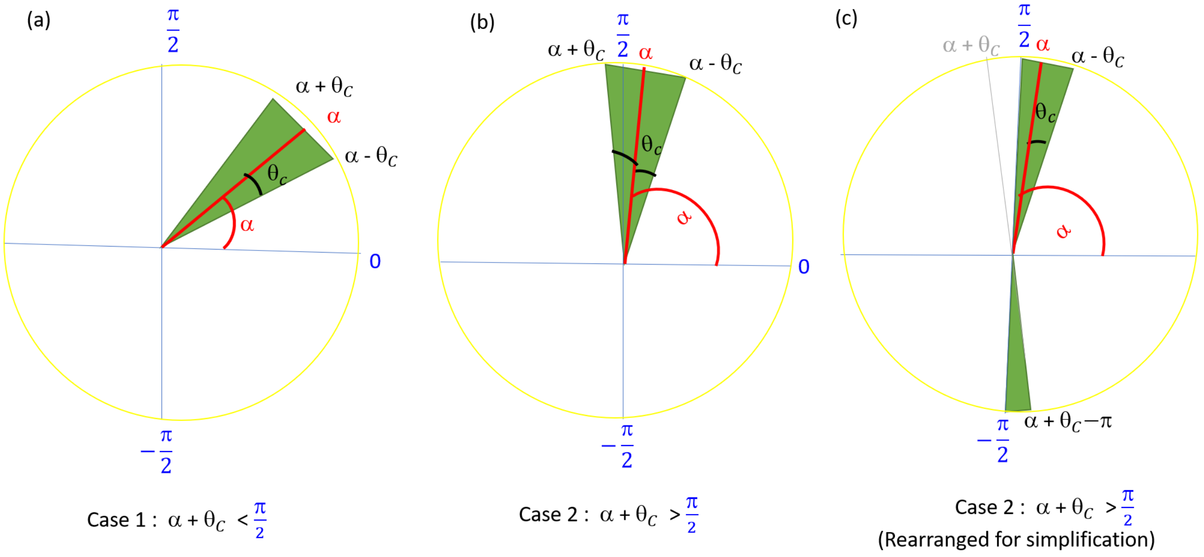


FIG. S1. Strain is applied at an angle $\alpha$, shown in red with respect to measurement direction at 0. The wire segements having angle lesser than the critical angle $\theta_C$ are broken with respect to strain direction, shown in green. (a) Represents the case 1 in which $\alpha + \theta_C < \frac{\pi}{2}$ and (b) represents the case 2 in which $\alpha + \theta_C > \frac{\pi}{2}$ and (c) is equivalent representation of case 2, with the rearrargement of broken region from second quadrant to fourth quadrant for simplification in calculations.

Here, we discuss resistance variation for strain along an arbitrary angle, $\alpha$ with respect to resistance measurement direction at an angle 0 (see Fig. S1). The strain breaks wire segments (edges), having an angle lesser than the critical angle, $\theta_C$ with respect to it. Thus, edges having angle $\alpha - \theta_C$ to $\alpha + \theta_C$ are broken as shown in the green region. The solution of resistance value is slightly tricky, solution for cases, $\alpha + \theta_C < \frac{\pi}{2}$ and $\alpha + \theta_C > \frac{\pi}{2}$ are different. Note that, as the wire segments are resistors, not like diodes, so the direction of current flowing through them depends on the polarity of the electric field and will be same if an edge is rotated by $\pi$. The potential difference across the edge, $V_i$, therefore depends on the orientation of edge as

$$V_i = EL_i|cos\theta_i| \tag{S1}$$

To avoid the issue of modulus in our calculations, for case 2, we rearrange the broken

region from the second quadrant to the fourth quadrant, where cosine is positive. Note that, in the main article, we studied the case of parallel and perpendicular strain in only first quadrant with angles 0 to $\frac{\pi}{2}$ due to symetery of the problem.

For case 1, $\alpha + \theta_C < \frac{\pi}{2}$:

As cosine is positive in first quadrent and hence it can be simply written as,

$$V_i = EL_i cos\theta_i \tag{S2}$$

If $\theta_C$ is critical angle such that wire segments below critical angle breaks down. Thus, average potential of all unbroken wire segments can be calculated as

$$V_{am} = \frac{\int_{-\frac{\pi}{2}}^{\alpha-\theta_C} EL_i cos\theta_i d\theta_i + \int_{\alpha+\theta_C}^{\frac{\pi}{2}} EL_i cos\theta_i d\theta_i}{\int_{-\frac{\pi}{2}}^{\alpha-\theta_C} d\theta_i + \int_{\alpha+\theta_C}^{\frac{\pi}{2}} d\theta_i} \tag{S3}$$

$$V_{am} = EL\,\frac{2 + sin(\alpha - \theta_C) - sin(\alpha + \theta_C)}{\pi - 2\theta_C} \tag{S4}$$

$$V_{am} = EL\,\frac{2 - 2\,cos\alpha\; sin\theta_C}{\pi - 2\theta_C} \tag{S5}$$

As discussed in the main article, the mean resistance of an individual edge is $\frac{\rho L_{am}}{wt}$ and the mean current through an edge is

$$I_{am} = \frac{Ewt}{\rho}\,\frac{2 - 2\,cos\alpha\; sin\theta_C}{\pi - 2\theta_C} \tag{S6}$$

The current across an equipotential line is

$$I_{eq} = \frac{Ewt}{\rho}\,\frac{2 - 2\,cos\alpha\; sin\theta_C}{\pi - 2\theta_C}\sqrt{N_u}b \tag{S7}$$

As the wire segments, with regions up-to angle $\theta_C$ are broken, i.e. $\sqrt{N_u} = \frac{\pi - 2\theta_C}{\pi}\sqrt{N}$.

By similar calulations provided in the main article,

$$R = \frac{R^0}{1 - \;cos\alpha\; sin\theta_C} \tag{S8}$$

One can arrive at special case of parallel strian discussed in main article, by substituting $\alpha = 0$ which matches exactly with the Eq. 7.

$$R^{\parallel} = \frac{R^0}{1 - sin\theta_C} \tag{S9}$$

For case 2, $\alpha + \theta_C > \frac{\pi}{2}$:

To avoid the issue of modulus, we rearrange the broken region from the second quadrant to fourth quadrant as cosine is positive in the fourth quadrant.

$$V_{am} = \frac{\int_{\alpha+\theta_C-\pi}^{\alpha-\theta_C} EL_i cos\theta_i d\theta_i}{\int_{\alpha+\theta_C-\pi}^{\alpha-\theta_C} d\theta_i} \tag{S10}$$

$$V_{am} = EL\,\frac{2 + sin(\alpha - \theta_C) + sin(\alpha + \theta_C)}{\pi - 2\theta_C} \tag{S11}$$

$$V_{am} = EL\,\frac{2\;sin\alpha\;cos\theta_C}{\pi - 2\theta_C} \tag{S12}$$

By similar calculations,

$$R = \frac{R^0}{sin\alpha\;cos\theta_C} \tag{S13}$$

One can arrive at special case of perpendicular strain, by substituting, $\alpha = \frac{\pi}{2}$ matching exactly with the Eq. 10 of the main article.

$$R^{\perp} = \frac{R^0}{cos\theta_C} \tag{S14}$$
